# Supplementary material for: New Wide Locally Recoverable Codes with Unified Locality
Source: arXiv:2505.06819 source file (2025-05-16)
Supplement: Supplementary file 1 [file appendix.tex]

\section{Appendix}
\subsection{The Code Rate Proof} \label{subsec:code_rate}
\begin{lemma}[The bounds on distance of UniLRC] \label{lemma:bo-UniLRC}
The distance of UniLRC(n, k, r, z) has a lower bound with
\[
d \geq \frac{n}{z} + 1 = r+2.
\]
\end{lemma}

\begin{proof}
The UniLRC can tolerate cluster-level failures while incurring zero cross-cluster traffic during single failure recovery. To maximize the code rate, it is essential to arrange each repair group within a single cluster and ensure that the number of symbols in any repair group does not exceed \( d-1 \). From this, we derive the inequality 
\[
r + 1 = \frac{n}{z} \leq d - 1,
\]
which completes the proof.
\end{proof}

\begin{theorem} \label{lemma:parity}
    For a UniLRC$(n, k, r, z)$ code, the number of parity symbols has the following lower bound:
\[
n - k \geq \frac{n}{z} + z - 1.
\]
If the code UniLRC$(n, k, r, z)$ meets the lower bound exactly, it will be an optimal LRC.
\end{theorem}
\begin{proof}
From Theorem 1, we know that
$$d \leq n - k - \left\lceil \frac{k}{r} \right\rceil + 2.$$
Let \( g \) denotes the number of global parities, and we have:
$$d \leq n - k - \left\lceil \frac{k}{r} \right\rceil + 2 = k + g + z - k - \left\lceil \frac{n - g - l}{r} \right\rceil + 2.$$
Simplifying this expression, we obtain:
\begin{equation} \label{equ:d_upper_bound}
d \leq g + z - \left\lceil \frac{n}{r} - \frac{g + z}{r} \right\rceil + 2 
%= g + z - \left\lceil \frac{z\times (r+1)}{r} - \frac{g + z}{r} \right\rceil + 2 
= g + 2 + \left\lfloor \frac{g+z}{r} \right\rfloor.
\end{equation}
Next, consider a repair group \( RG = \{c_1, \ldots, c_r, c_{r+1}\} \), where \( c_i \) represents a symbol. Then \( RG = c_l \cup B \), where \( B \) is the set of MDS symbols and $c_l$ is the local parity. To tolerate a repair group failure, we must ensure that \( |B| \leq g \). Thus, we have:
$$|RG| = r + 1 \leq g + 1.$$
That implies:
\begin{equation} \label{equ:rlessthang}
    r \leq g.
\end{equation}
Combined equations \ref{equ:d_upper_bound} and \ref{equ:rlessthang}, we obtain the following bound:
\begin{equation} \label{equ:upper_bound}
 n - k - \left\lceil \frac{k}{r} \right\rceil + 2 = 
g + 2 + \left\lfloor \frac{g+z}{r} \right\rfloor \geq g + 3.
\end{equation}
From Lemma \ref{lemma:bo-UniLRC}, we know that \( d \geq \frac{n}{z} + 1 = r + 2 \). Combined this with inequation \ref{equ:rlessthang}, we get: 
\begin{equation} \label{equ:low_bound}
    \frac{n}{z} + 1 \leq g + 2.
\end{equation}
Therefore, from the derived lower and upper bounds, we have:
\[
\frac{n}{z} + 1 \leq d \leq n - k - \left\lceil \frac{k}{r} \right\rceil + 2.
\]
However, the equalities derived from inequalities \ref{equ:upper_bound} and \ref{equ:low_bound} cannot be satisfied simultaneously. Therefore, we conclude that:
\[
n - k - \left\lceil \frac{k}{r} \right\rceil + 2 > \frac{n}{z} + 1,
\]
which simplifies to:
\[
n - k + 1 > \frac{n}{z} + \left\lceil \frac{k}{r} \right\rceil,
\]
leading to the final inequality:
\begin{equation} \label{equ:z}
n - k \geq \frac{n}{z} + \left\lceil \frac{k}{r} \right\rceil.
\end{equation}
Given that $g+k+l = z(r+1)$, and with exactly $z$ local groups, and we can deduce: 
\begin{equation}\label{equ:x}
    g+k = zr.
\end{equation}

From inequation \ref{equ:rlessthang},  to achieve the smallest global parity redundancy, we require $r=g$. 
Combined this with equation \ref{equ:x}, we obtain: 
\begin{equation}\label{equ:s}
    k = (z-1)r.
\end{equation}
Then, 
\begin{equation} \label{equ:h}
n - k \geq \frac{n}{z} + z - 1.
\end{equation}
We complete the proof.
\end{proof}

% \begin{theorem}
%     If a good UniLRC is an optimal LRC, its minimum distance must satisfy the following equation:
%     $$d = g+2.$$
% \end{theorem}

% \begin{proof}
%     Next, we demonstrate that the equality in inequality \ref{equ:z} is equivalent to the equation \ref{equ:bound_of_optimal_lrc} as presented in Lemma \ref{lemma:other_singleton}. Specifically, we have:
% \begin{equation} \label{equ:q}
%     n - k = \frac{n}{z} + z - 1 = z + r = g + \frac{n}{r+1} = d-2 + \frac{n}{r+1},
% \end{equation}
% which satisfies the condition of Corollary \ref{coro:other_singleton}.
% \end{proof}

\begin{corollary}[UniLRC code rate bound]
The rate of a UniLRC$(n, k, r, z)$ code satisfies
\[
\frac{k}{n} \leq \frac{r}{r+1} (1-\frac{1}{z}).
\]
\end{corollary}

\begin{proof}
The proof is straightforward by Theorem \ref{lemma:parity} and $n=z(r+1)$, and we can simplify as follows: 
\[
\frac{k}{n} \leq \frac{r}{r+1} (1-\frac{1}{z}).
\]

If we let $z = 1$, this implies that there is only one cluster, which cannot tolerate cluster-level failures. Therefore, in all other cases where $z - 1 > 0$, the code rate bound is positively correlated with both the number of clusters and the size of the repair group.
\end{proof}

\subsection{Distance Proof}
\begin{theorem} \cite{huffman2010fundamentals} \label{thm:gen_parity_check}
    If 
    $G = \left[\begin{array}{c|c}
        I_k & A
    \end{array}\right] $
    is a generator matrix for the [n, k] code C in standard form, then $H = \left[\begin{array}{c|c}
        -A^\top & I_{n-k}
    \end{array}\right] $
    is a parity check matrix for C.
\end{theorem} 

\begin{theorem} \label{thm:distance_app}
    The UniLRC(n, k, r, z) possesses a minimum distance of precisely $g+2$, making it the optimal LRC..
\end{theorem}

\begin{proof}
    From the generator matrix of Sec \ref{equ:construction_unilrc} and Theorem \ref{thm:gen_parity_check}, we can get the parity matrix 
    $H = \left[\begin{array}{c|c}
        A & I_{n-k}
    \end{array}\right] $
    and 
    $A = \left[\begin{array}{c}
        \mathcal{G}  \\
        \hline
        \mathcal{L}
    \end{array}\right], $ where 
$$
\mathcal{G}=
\begin{bmatrix}
    1 & 1 & ... & 1 \\
    g_1 & g_2 & ... & g_k \\
    ... & ... & ... & ... \\
    g_1^{z-1} & g_2^{z-1} & ... & g_k^{z-1} \\
    g_1^{z} & g_2^{z} & ... & g_k^{z}
\end{bmatrix},$$
$$
\mathcal{L} = \begin{bmatrix}
    s_{1,1} + l_1 & s_{1,2} & ... & s_{1,k} \\
     s_{1,1} & s_{1,2} + l_2 & ... & s_{1,k} \\
    ... & ... & ... & ... \\
    s_{z,1} & s_{z,2} & ... & s_{z,k} + l_z \\
\end{bmatrix}.
$$
% We assume that the code has $z+1$ failures, where $A$ has $f$ failures and $I_{n-k}$ has the remaining $z+1-f$ failures.
% Next, the system can recover from up to $z+1$ failures, which corresponds to solving the equation $Ax = b$ where the system of linear equations has a unique solution.

Next, we will prove \textbf{\textit{the parity check matrix $H$ has a set of $g+2$ linearly dependent columns but no set of $g + 1$ linearly dependent columns}}.

First, we prove any $g + 1$ columns are linearly independent.
To show the process clearly, we split $H$ as three parts:  
$$ H =
\left [ \begin{array}{c|c|c}
    A & I_{G} & I_{L}
\end{array} \right], 
$$
where $I_{G}$ and $I_{L}$ represents the coefficients of global parity and local parity, respectively.
We assume that the $g + 1$ columns consist of $A, I_{G}$ and $I_{L}$, where it chooses $a,b$ and $c$ columns from $A, I_{G}$ and $I_{L}$, respectively.
Then, there are multiple cases for $a, b$ and $c$.

(1) If $a = g+1, b=c=0$, we show the vectors chosen as matrix $T$ as following:
$$ T =
\left [ \begin{array}{cccc}
    v_{1,1} & v_{1,2} & ... & v_{1,g+1} \\
    v_{2,1} & v_{2,2} & ... & v_{2,g+1} \\
    {...}   & {...}   & ... & {...} \\
    v_{g,1} & v_{g,2} & ... & v_{g,g+1} \\
    \hline
    s_{1,1} + l_1 & s_{1,2} & ... & s_{1,g+1} \\
     s_{1,1} & s_{1,2} + l_2 & ... & s_{1,g+1} \\
    ... & ... & ... & ... \\
    s_{z,1} & s_{z,2} & ... & s_{g,g+1} + l_z \\  
\end{array} \right].
$$
And we can simplify $T$ by elementary transformation as following:
$$
\left [ \begin{array}{cccc}
    v_{1,1} & v_{1,2} & ... & v_{1,g+1} \\
    v_{2,1} & v_{2,2} & ... & v_{2,g+1} \\
    {...}   & {...}   & ... & {...} \\
    v_{g,1} & v_{g,2} & ... & v_{g,g+1} \\
    \hline
    v_{g+1,1} & v_{g+1,2} & ... & v_{g+1,g+1} \\
    {0}   & {0}   & ... & {0} \\
    {...}   & {...}   & ... & {...} \\
    {0}   & {0}   & ... & {0} \\ 
\end{array} \right]
= 
\left [ \begin{array}{c}
    V \\
    \hline
    O
\end{array} \right],
$$
where $V$ is the Vandermonde matrix and $O$ is zero matrix. Therefore, the $rank(T) = rank(V) = g + 1$, which proves the $g+1$ columns are linear independent.

(2) If $c=0, a + b = g+1$ and $b \neq 0$, we show the vectors chosen as matrix $T$ as following:
$$ 
\left [ \begin{array}{cccc |cccc} \tiny
    v_{1,1} & v_{1,2} & ... & v_{1,a} & 1 & 0 & ... & 0\\
    v_{2,1} & v_{2,2} & ... & v_{2,a} & 0 & 1 & ... & 0\\
    {...}   & {...}   & ... & {...} & {...}   & {...}   & ... & {...}\\
    v_{g,1} & v_{g,2} & ... & v_{g,a} & 0 & 0 & ... & 1\\
    \hline
    s_{1,1} + l_{1,1}  & s_{1,2} & ... & s_{1,a} & 0 & 0 & ... & 0\\
    s_{2,1} & s_{2,2} + l_{1,2} & ... & s_{1,a} & 0 & 0 & ... & 0\\
    {...}   & {...}   & ... & {...} & {...}     & {...}   & ... & {...}\\
    s_{g,1} & s_{g,2} & ... & s_{g,a} + l_{1,a} & 0 & 0 & ... & 0\\    
\end{array} \right].
$$
And we can simplify $T$ by elementary transformation as following:
$$
\left [ \tiny \begin{array}{cccc |cccc}
    v_{1,1} & v_{1,2} & ... & v_{1,a} & 0 & 0 & ... & 0\\
    v_{2,1} & v_{2,2} & ... & v_{2,a} & 0 & 0 & ... & 0\\
    {...}   & {...}   & ... & {...} & {...}   & {...}   & ... & {...}\\
    v_{g+1,1} & v_{g+1,2} & ... & v_{g+1,a} & 0 & 0 & ... & 0\\
    \hline
    0  & 0 & ... & 0 & 1 & 0 & ... & 0\\
    0  & 0 & ... & 0  & 0 & 1 & ... & 0\\
    {...}   & {...}   & ... & {...} & {...}   & {...}   & ... & {...}\\
    0  & 0 & ... & 0 & 0 & 0 & ... & 1\\    
\end{array} \right]
= 
\left [ \begin{array}{c|c}
    V_a & O\\
    \hline
    O & I_{b}
\end{array} \right],
$$
where $v_a$ is Vandermonde with $a$ columns and $I_b$ is $b\times b$ identify matrix. Therefore, the $rank(T) = rank(V_a) + rank(I_b) = a + b = g + 1$, which proves the $g+1$ columns are linear independent.

(3) If $a + b + c = g+1$ and $a \neq 0, b\neq 0, c\neq 0$, we show the vectors chosen as matrix $T$ as following:
$$
\left [ \tiny \begin{array}{cccc |cccc|cccc} 
    v_{1,1} & v_{1,2} & ... & v_{1,a} & 1 & 0 & ... & 0& 0 & 0 & ... & 0\\
    v_{2,1} & v_{2,2} & ... & v_{2,a} & 0 & 1 & ... & 0& 0 & 0 & ... & 0\\
    {...}   & {...}   & ... & {...} & {...}   & {...}   & ... & {...} &{...}   & {...}   & ... & {...}\\
    v_{g,1} & v_{g,2} & ... & v_{g,a} & 0 & 0 & ... & 1& 0 & 0 & ... & 0\\
    \hline
    s_{1,1} + l_{1,1}  & s_{1,2} & ... & s_{1,a} & 0 & 0 & ... & 0 & 1 & 0 & ... & 0\\
    s_{2,1} & s_{2,2} + l_{1,2} & ... & s_{1,a} & 0 & 0 & ... & 0 & 0 & 1 & ... & 0\\
    {...}   & {...}   & ... & {...} & {...}   & {...}   & ... & {...} &{...}   & {...}   & ... & {...}\\
    s_{g,1} & s_{g,2} & ... & s_{g,a} + l_{1,a} & 0 & 0 & ... & 0 & 0 & 0 & ... & 1\\    
\end{array} \right].
$$
And we can simplify $T$ by elementary transformation as following:
$$
\left [ \tiny\begin{array}{cccc |cccc |cccc }
    v_{1,1} & v_{1,2} & ... & v_{1,a} & 0 & 0 & ... & 0 & 0 & 0 & ... & 0\\
    v_{2,1} & v_{2,2} & ... & v_{2,a} & 0 & 0 & ... & 0 & 0 & 0 & ... & 0\\
    {...}   & {...}   & ... & {...} & {...}   & {...}   & ... & {...} & {...}   & {...}   & ... & {...}\\
    v_{g+1,1} & v_{g+1,2} & ... & v_{g+1,a} & 0 & 0 & ... & 0 & 0 & 0 & ... & 0\\
    \hline
    0  & 0 & ... & 0 & 1 & 0 & ... & 0 & 0 & 0 & ... & 0\\
    0  & 0 & ... & 0  & 0 & 1 & ... & 0 & 0 & 0 & ... & 0\\
    {...}   & {...}   & ... & {...} & {...}   & {...}   & ... & {...} & {...}   & {...}   & ... & {...}\\
    0  & 0 & ... & 0 & 0 & 0 & ... & 1 & 0 & 0 & ... & 0\\    
    \hline
     0  & 0 & ... & 0 & 0 & 0 & ... & 0 & 1 & 0 & ... & 0\\
    0  & 0 & ... & 0  & 0 & 0 & ... & 0 & 0 & 1 & ... & 0\\
    {...}   & {...}   & ... & {...} & {...}   & {...}   & ... & {...} &{...}   & {...}   & ... & {...}\\
    0  & 0 & ... & 0 & 0 & 0 & ... & 0 & 0 & 0 & ... & 1\\ 
\end{array} \right]
$$
$$
= 
\left [ \begin{array}{c|c|c}
    V_a & O & O\\
    \hline
    O & I_{b} & O \\
    \hline 
    O & O & I_{c} 
    
\end{array} \right],
$$
where $v_a$ is Vandermonde matrix with $a$ columns and $I_b, I_c$ is $b\times b, c\times c$ identify matrix's, respectively.
Therefore, the $rank(T) = rank(V_a) + rank(I_b) + rank(I_c)= a + b + c= g + 1$, which proves the $g+1$ columns are linear independent.

Second, it is easy to give an example to show the $g+2$ columns are linearly dependent. Take the example of (1), if we add a new information column, we can get $T$ as following:
$$ T =
\left [ \begin{array}{c}
    G' \\
    \hline
    L'
\end{array} \right]
=
\left [ \tiny \begin{array}{ccccc}
    v_{1,1} & v_{1,2} & ... & v_{1,g+1} & \mathbf{v_{1,g+2}}\\
    v_{2,1} & v_{2,2} & ... & v_{2,g+1} & \mathbf{v_{1,g+1}}\\
    {...}   & {...}   & ... & {...} & {...}  \\
    v_{g,1} & v_{g,2} & ... & v_{g,g+1} & \mathbf{v_{g,g+2}}\\
    \hline
    v_{1,1} + l_{1,1}  & v_{1,2} & ... & v_{1,g+1} & \mathbf{v_{1,g+2}}\\
    v_{2,1} & v_{2,2} + l_{1,2} & ... & v_{1,g+1} & \mathbf{v_{2,g+2}}\\
    {...}   & {...}   & ... & {...} & {...} \\
    v_{g,1} & v_{g,2} & ... & v_{g,g+1} + l_{1,g+1} & \mathbf{v_{g,g+2}}\\    
\end{array} \right].
$$
And we can simplify $T$ by elementary transformation as following:
$$
\left [ \begin{array}{ccccc}
    v_{1,1} & v_{1,2} & ... & v_{1,g+1} & \mathbf{v_{1,g+2}}\\
    v_{2,1} & v_{2,2} & ... & v_{2,g+1} & \mathbf{v_{2,g+2}}\\
    {...}   & {...}   & ... & {...} & {...}\\
    v_{g,1} & v_{g,2} & ... & v_{g,g+1} & \mathbf{v_{g,g+2}}\\
    \hline
    v_{g+1,1} & v_{g+1,2} & ... & v_{g+1,g+1} & \mathbf{v_{g+1,g+2}}\\
    {0}   & {0}   & ... & {0} & {0} \\
    {...}   & {...}   & ... & {...} & {...}\\
    {0}   & {0}   & ... & {0} & {0} \\ 
\end{array} \right]
= 
\left [ \begin{array}{c}
    V' \\
    \hline
    O
\end{array} \right],
$$
where $V$ is the Vandermonde matrix and $O$ is zero matrix. However, the $rank(T) = rank(V') = g + 1$, so the $g + 2$ columns must be linearly independent.

In summary, we give the proof of parity check matrix $H$ with \textbf{$g+2$ linearly dependent columns} but \textbf{any $g + 1$ columns are linearly independent}. So the distance is exactly $g+2$.

By organizing one repair group into a cluster, we deduce that $\frac{n}{r+1} = l$. Incorporating this into Corollary \ref{coro:other_singleton} with the minimum distance $d = g+2$, we ultimately derive the optimal LRC configuration.
\end{proof}
